# Supplementary material for: Infrared spectra in amorphous alumina: a combined ab initio and experimental study
Source: arXiv:2304.14090 source file (2023-04-27)
Supplement: Supplementary file 1 [file supplement.pdf]

# **Infrared spectra in amorphous alumina: a combined *ab-initio* and experimental study**

**Luigi Giacomazzi**

Institute of Materials (IOM), National Research Council of Italy (CNR), c/o SISSA Via Bonomea 265, IT-34136 Trieste, Italy  
Materials Research Laboratory, University of Nova Gorica, Vipavska 11c, SI-5270 Ajdovščina, Slovenia

**Nikita S. Shcheblanov**

Navier, UMR 8205, Ecole des Ponts ParisTech, Univ. Gustave Eiffel, CNRS, Marne-la-Vallée, France and MSME, UMR 8208, Univ. Gustave Eiffel, CNRS, Univ. Paris-Est Créteil, Marne-la-Vallée, France

**Mikhail E. Povarnitsyn**

Joint Institute for High Temperatures, RAS, 13 Building 2 Izhorskaya Street, Moscow 125412, Russia

**Yanbo Li**

Institute of Fundamental and Frontier Sciences, University of Electronic Science and Technology of China, Chengdu, 610054 China

**Andraž Mavrič**

Materials Research Laboratory, University of Nova Gorica, Vipavska 11c, SI-5270 Ajdovščina, Slovenia

**Barbara Zupančič and Jože Grdadolnik**

Laboratory for Molecular Structural Dynamics, Theory Department, National Institute of Chemistry, 1000 Ljubljana, Slovenia

**Alfredo Pasquarello**

Chaire de Simulation à l'Echelle Atomique (CSEA), Ecole Fédérale Polytechnique de Lausanne (EPFL), CH-1015 Lausanne, Switzerland

### Thin-film characterization

Cross-sectional specimens for Transmission Electron Microscopy (TEM) observations were prepared by cutting the thin-film coated substrate along the thickness direction. The cross-section was glued with epoxy resin and processed employing a standard mechanical sample preparation process and finalized by Ar-ion milling and polishing (PIPS II, GATAN) at grazing incidence  $<5^\circ$ . The acceleration voltage for TEM was 100 kV (JEOL JEM2100F) to prevent beam-induced crystallization [[10.1016/j.jnoncrysol.2018.07.055](https://doi.org/10.1016/j.jnoncrysol.2018.07.055)]. X-ray diffraction (XRD) and X-ray reflectivity (XRR) measurements were taken on Rigaku SmartLab SE with  $\text{CuK}\alpha$  source (2.2 kW).

XRR data for  $\text{Al}_2\text{O}_3$  thin film on Si were collected on a 100 nm thick film due to the limit in the instrument resolution. Fitting the reflectivity curve was done using the Smart Lab Studio II (Rigaku) software package. The film demonstrates a low surface roughness of 1.1 nm and a density of 2.74 g/cm<sup>3</sup> [Fig. S1(a)].

TEM images show a homogenous and void-free  $\text{Al}_2\text{O}_3$  thin film on a Si substrate [Fig. S1(c)]. A high-resolution TEM image shows the amorphous nature of  $\text{Al}_2\text{O}_3$  on crystalline Si, separated by an approximately 2 nm thick  $\text{SiO}_2$  layer [Fig. S1(d)]. The amorphous nature was also confirmed by the absence of Bragg diffraction peaks in the XRD pattern [Fig. S1(b)], measured in a parallel beam geometry with Si (111) peak misaligned by  $2^\circ$ . The blue line marks the diffraction on substrate surface truncation at  $28.4^\circ$ .

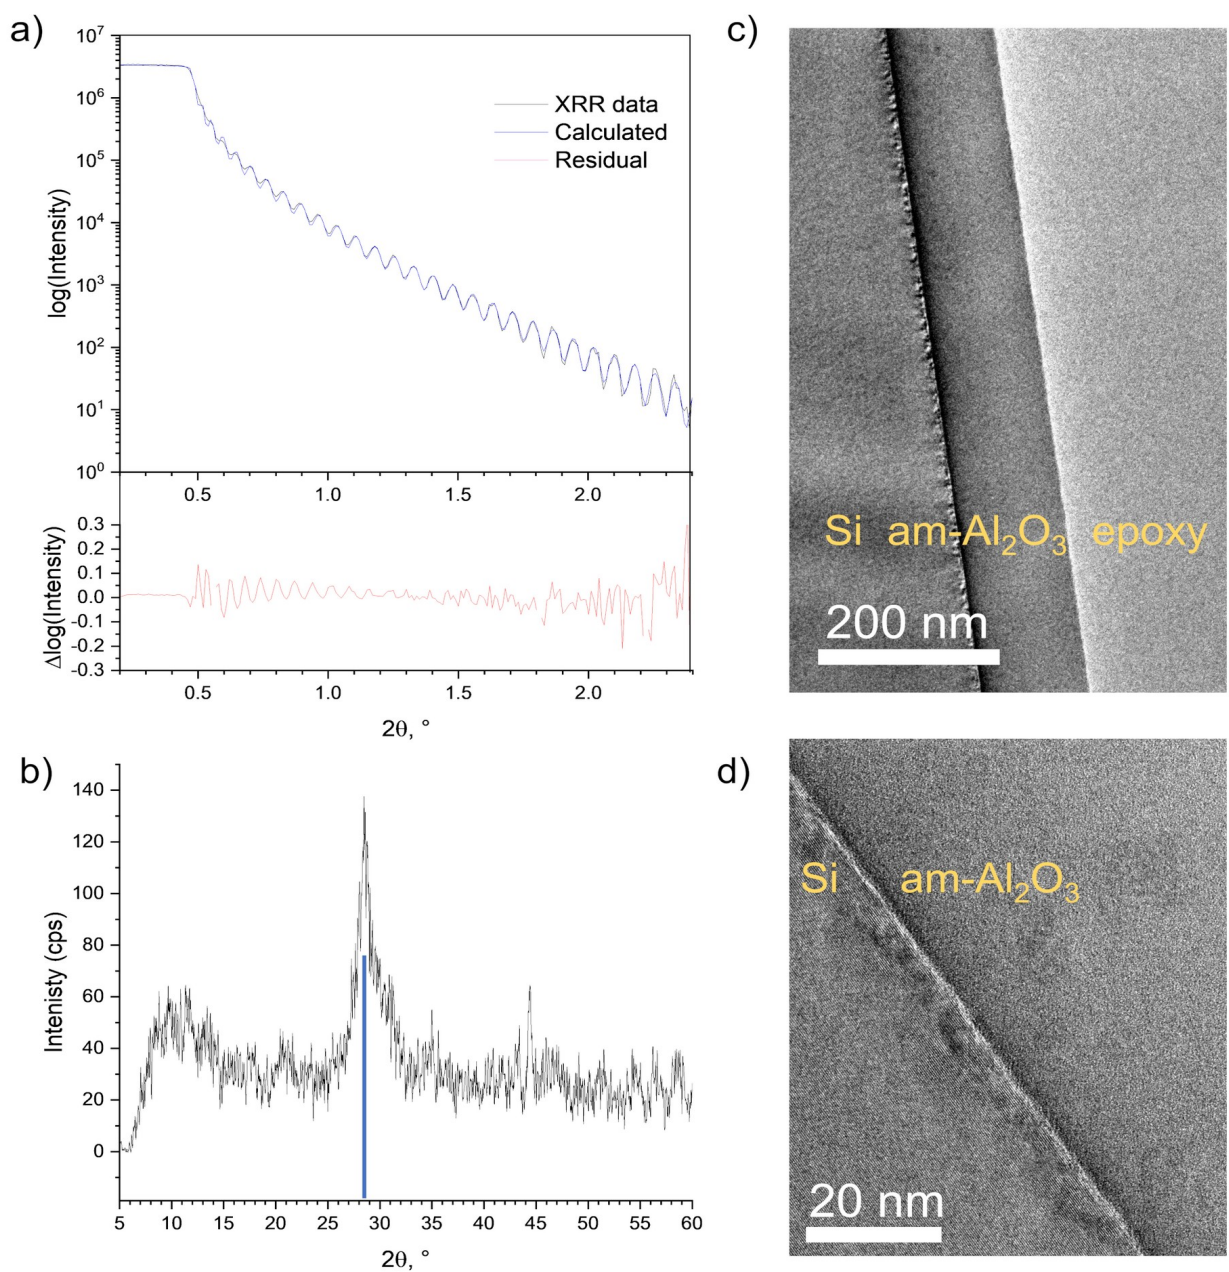

Figure S1

- XRR measurement of 100 nm  $\text{Al}_2\text{O}_3$  thin film on Si with fitted oscillation model.
- XRD pattern of 300 nm  $\text{Al}_2\text{O}_3$  thin film on Si, measured in a parallel beam geometry with Si (111) peak misaligned by  $2^\circ$ , the blue line indicates Si surface truncation
- TEM image of  $\text{Al}_2\text{O}_3$  thin film cross-section
- HR-TEM image of  $\text{Al}_2\text{O}_3$  showing monocrystalline Si wafer and amorphous, void-free coating.

### am-Al<sub>2</sub>O<sub>3</sub> vibrational analysis: participation ratio

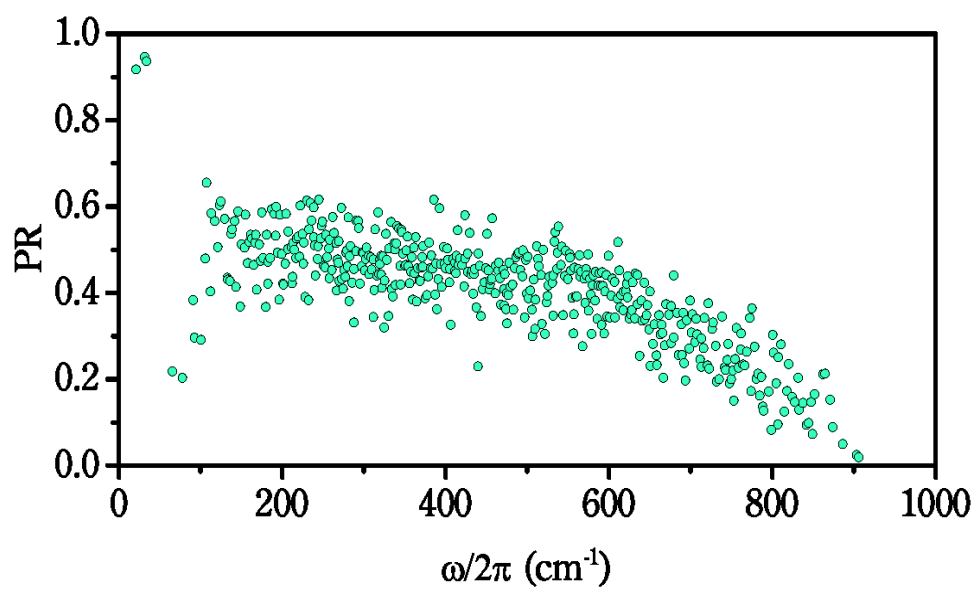

Figures S2: Participation ratio as calculated for the vibrational modes of model I of am-Al<sub>2</sub>O<sub>3</sub>. It can be noted that the modes between 200 and 400 cm<sup>-1</sup> are not spatially localized on individual OAl<sub>3</sub> units, while the stretching modes above 500 cm<sup>-1</sup> show a tendency to become much more spatially localized.

## IR active modes in $\theta$ -alumina

We have calculated, as explained in the method section, the vibrational modes and frequencies in a supercell of 200 atoms of  $\theta$ -alumina [Z. Lodziana and K. Parlinski, Phys. Rev. B **67**, 174106 (2003)] and compared the location of the relevant IR modes to the experimental results of Fig. 6 of [A. Boumaza *et al*, J. Solid State Chem. **182**, 1171 (2009)]. Apart from the underestimation of the peak positions of about  $40\text{ cm}^{-1}$ , the result of our calculation are consistent with the experimental findings, in particular for the location of the peculiar doublet at  $330$  and  $370\text{ cm}^{-1}$  and for the doublet at  $760$  and  $820\text{ cm}^{-1}$ . We note that also the preliminary B3LYP-DFT calculations of Boumaza *et al.* underestimate the frequency position of the doublet locating it at about  $300\text{ cm}^{-1}$ .

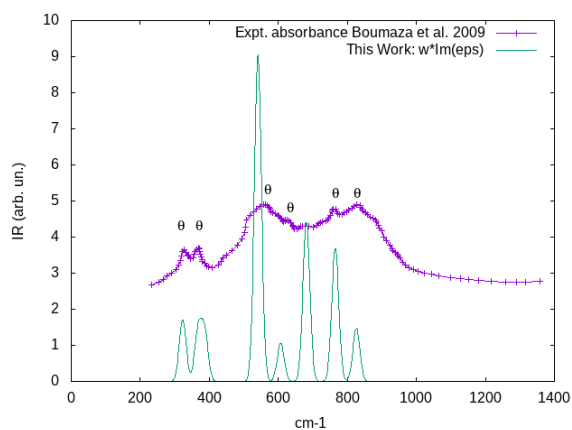

Figure S3: Comparison of the experimental IR absorbance as measured in Fig.6 of Boumaza *et al* J. Solid State Chem. **182**, 1171 (2009) versus  $\omega \cdot \text{Im}(\epsilon)$  spectrum for the 200 atoms supercell calculated from first-principles. A rigid shift of  $40\text{ cm}^{-1}$  was applied to the calculated frequencies

Direct inspection, using the visualization software Xcrysden (<http://www.xcrysden.org/>) shows that the vibrational modes underlying the doublet at  $285$  and  $330\text{ cm}^{-1}$  exhibit a remarkable *out-of-plane* motion of threefold oxygen atoms.

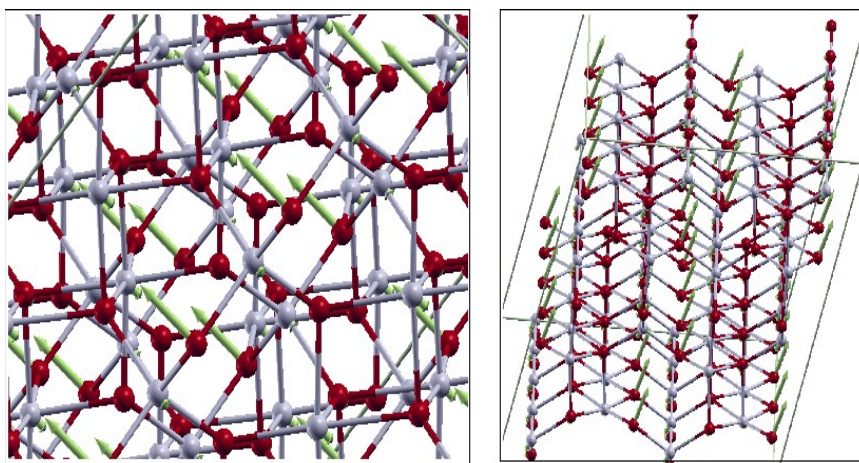

Figure S4: Vibrational modes at about  $285\text{ cm}^{-1}$  (left panel) and at about  $330\text{ cm}^{-1}$  (right panel) featuring out-of-plane motion of threefold oxygen atoms as calculated for a 200 atom supercell of  $\theta$ -alumina.
